# Supplementary material for: Dataset-Agnostic Recommender Systems
Source: arXiv:2501.07294 source file (2025-04-23)
Supplement: Supplementary file 1 [file neurips_appendix.tex]

\section{Technical Appendices and Supplementary Material}
Technical appendices with additional results, figures, graphs and proofs may be submitted with the paper submission before the full submission deadline (see above), or as a separate PDF in the ZIP file below before the supplementary material deadline. There is no page limit for the technical appendices.

%%%%%%%%%%%%%%%%%%%%%%%%%%%%%%%%%%%%%%%%%%%%%%%%%%%%%%%%%%%%

\newpage
